# Supplementary material for: HCSC: Hierarchical Contrastive Selective Coding
Source: arXiv:2202.00455 source file (2022-05-23)
Supplement: Supplementary file 1 [file supp.tex]

% CVPR 2022 Paper Template
% based on the CVPR template provided by Ming-Ming Cheng (https://github.com/MCG-NKU/CVPR_Template)
% modified and extended by Stefan Roth (stefan.roth@NOSPAMtu-darmstadt.de)

\documentclass[10pt,twocolumn,letterpaper]{article}

%%%%%%%%% PAPER TYPE  - PLEASE UPDATE FOR FINAL VERSION
\usepackage[review]{cvpr}      % To 
\usepackage{graphicx}
\usepackage{amsmath}
\usepackage{amssymb}
\usepackage{booktabs}
\usepackage{setspace}
\usepackage{algorithmic}
\usepackage{algorithm}
\usepackage{bbm}
\usepackage[pagebackref,breaklinks,colorlinks]{hyperref}

% Support for easy cross-referencing
\usepackage[capitalize]{cleveref}
\crefname{section}{Sec.}{Secs.}
\Crefname{section}{Section}{Sections}
\Crefname{table}{Table}{Tables}
\crefname{table}{Tab.}{Tabs.}

% For pseudo codes

%%%%%%%%% PAPER ID  - PLEASE UPDATE
 % *** Enter the CVPR Paper ID here

\begin{document}

%%%%%%%%% TITLE - PLEASE UPDATE

\title{HCSC: Hierarchical Contrastive Selective Coding \\ \emph{Supplementary Material}}
\maketitle
\input{tex/appendix.tex}

\newpage
\small
\bibliographystyle{ieee_fullname}
\bibliography{egbib}

\end{document}
